# Supplementary material for: REVEAL: Retrieval-Augmented Visual-Language Pre-Training with Multi-Source Multimodal Knowledge Memory
Source: arXiv:2212.05221 source file (2023-04-03)
Supplement: Supplementary file 1 [file appendix.tex]

\section{More Qualitative Examples}
We show examples of visual question answering and image captions in Figure~\ref{fig:correct_vqa}-\ref{fig:caption}.

\begin{figure*}
    \includegraphics[width=0.9\columnwidth]{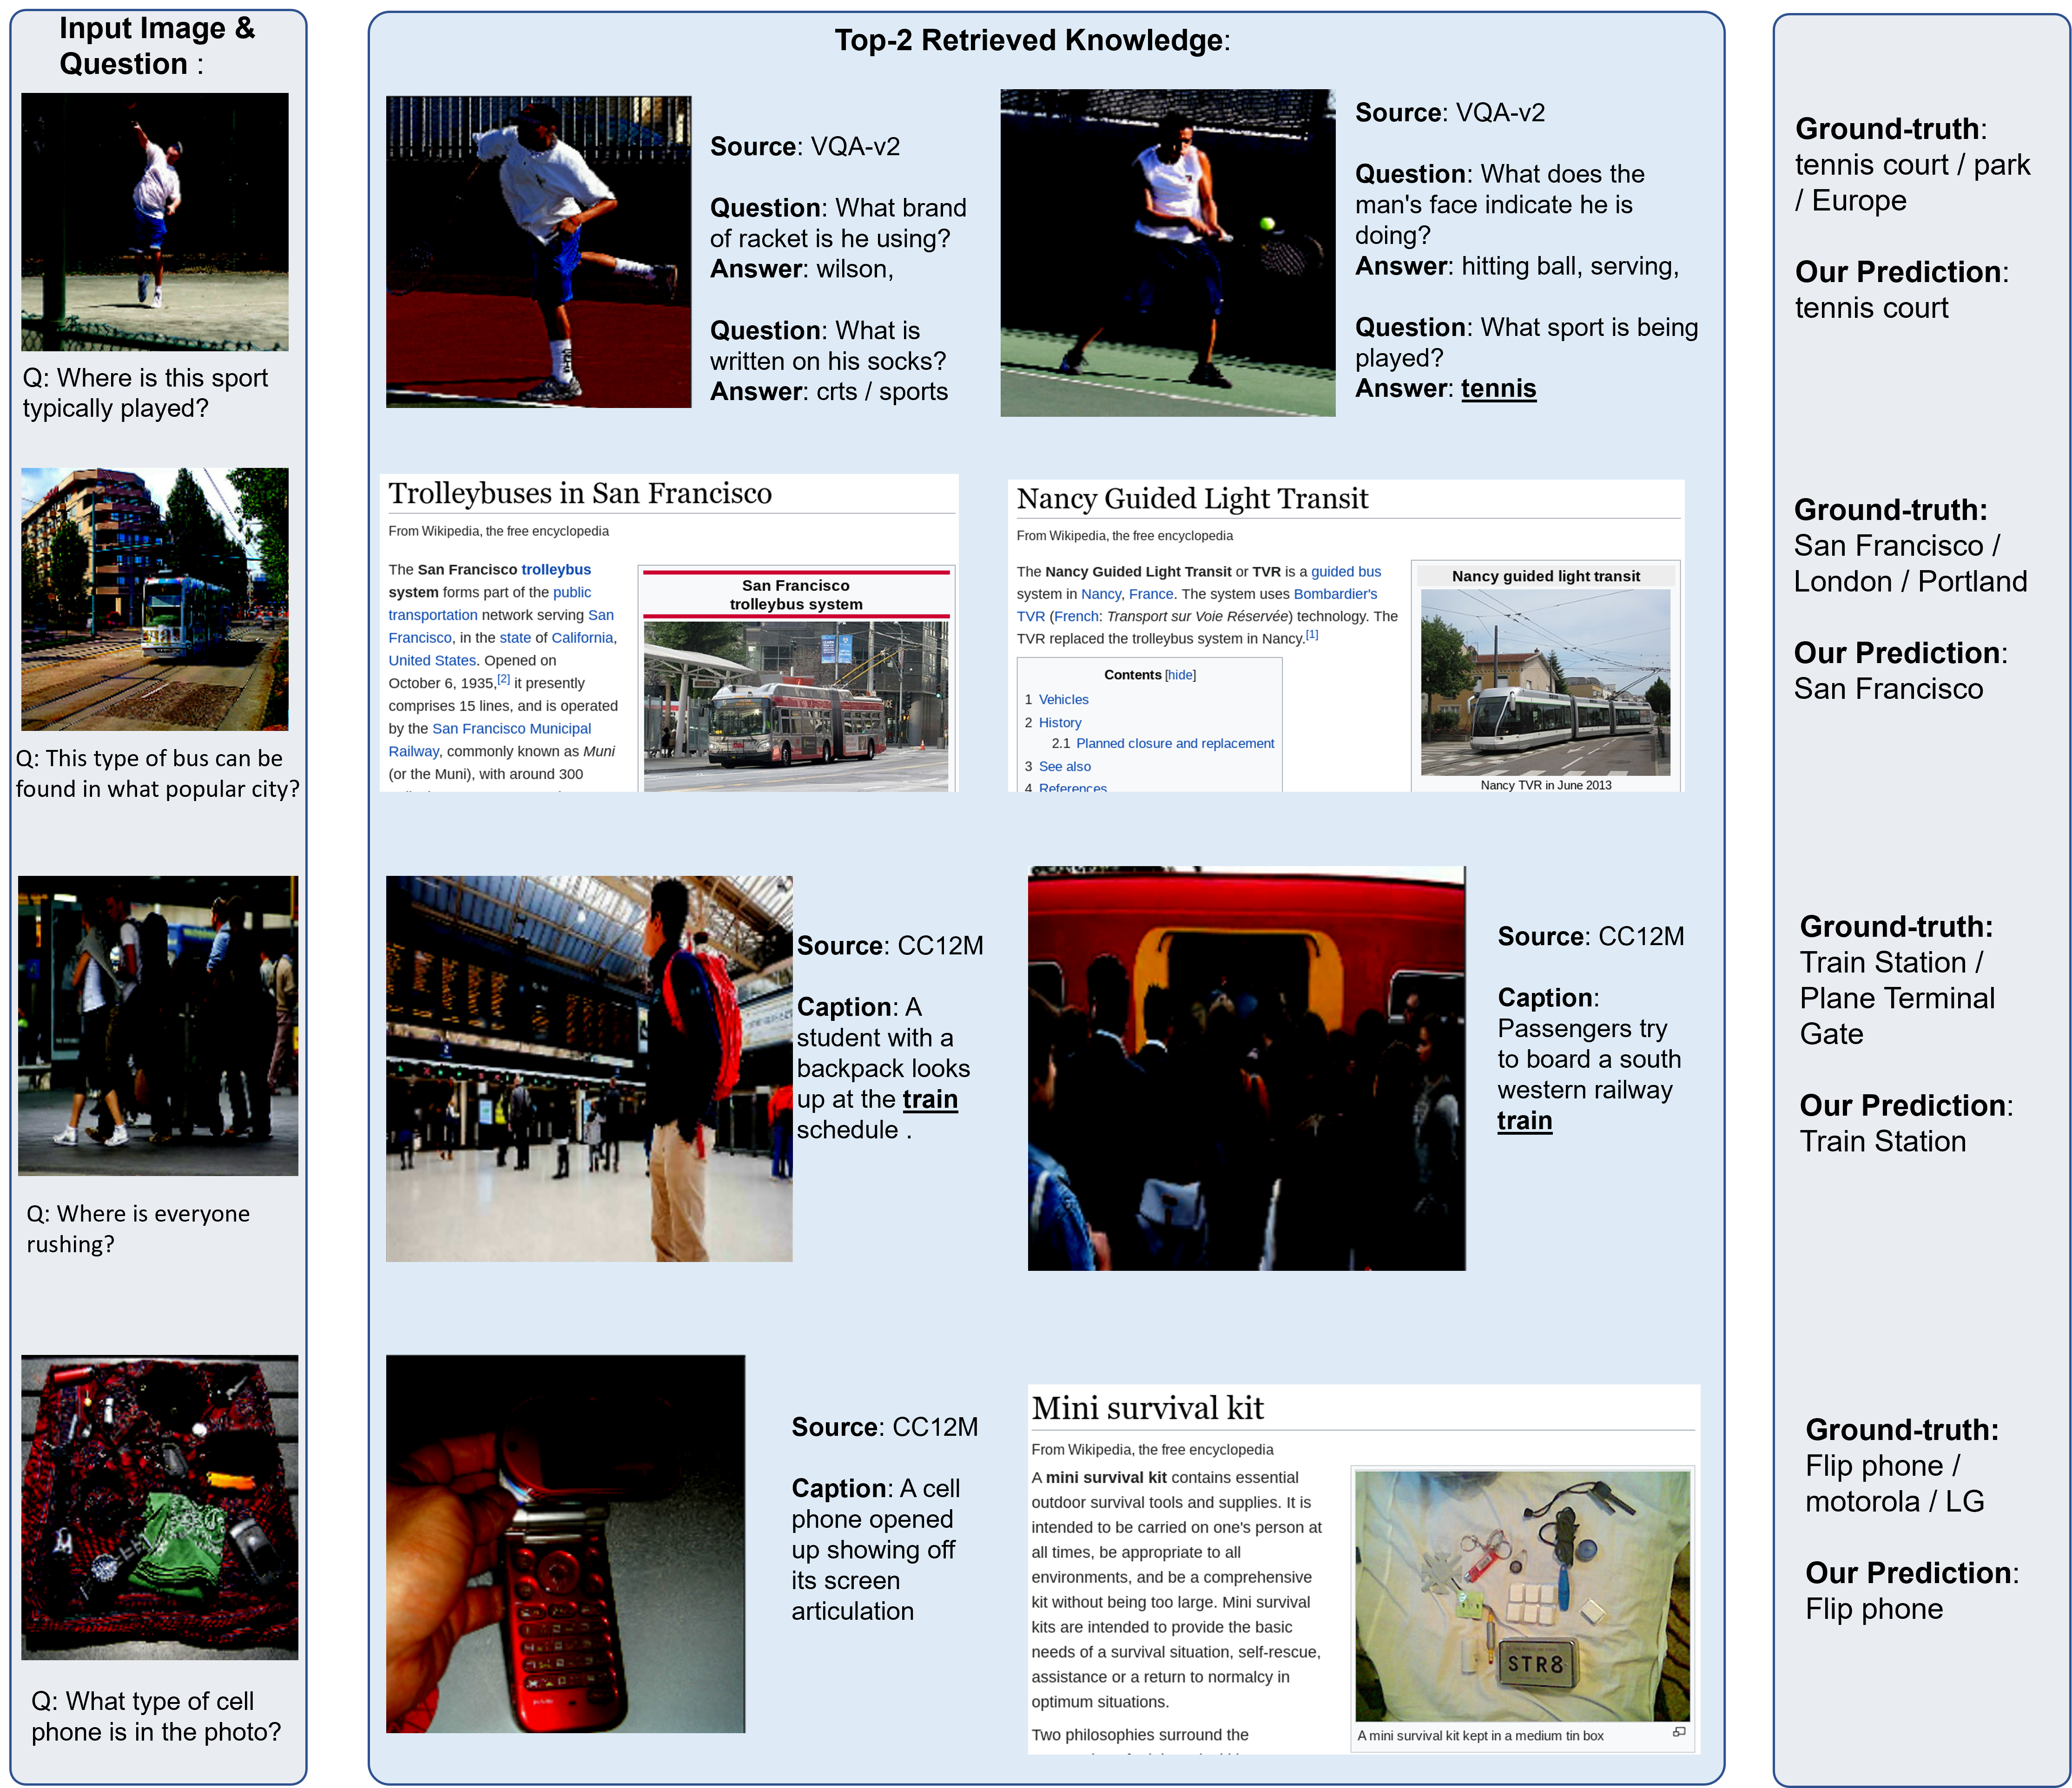}
    \captionof{figure}{Examples of VQA pairs from OKVQA benchmark that \method correctly generate the answer.}
    \label{fig:correct_vqa}
\end{figure*}

For visual question answering, we select four examples that correctly answer the question in Figure~\ref{fig:correct_vqa}, and three examples that our model predicts wrongly. For both cases, the \method could learn to retrieve relevant information from diverse knowledge sources. For example, in the first question in Figure~\ref{fig:correct_vqa}, \method retrieves two VQA pairs from VQA-v2 datasets relevant to tennis playing to provide information, and in the second question \method correctly retrieves the Wikipedia page about trolleybus in San Francisco to answer where the bus might appear. The third example utilizes the image caption pairs from CC12M, which encodes the commonsense knowledge that a crowd of people might indicate they are rushing towards the train station to catch up deadline. These examples show that the corpus gating module in \method could help identify the most useful knowledge source for different questions. In addition, the Top-100 retrieved knowledge might come from different knowledge sources, and the model could jointly reason with these diverse knowledge entries to get correct answers.

\begin{figure*}
    \centering
    \includegraphics[width=0.9\columnwidth]{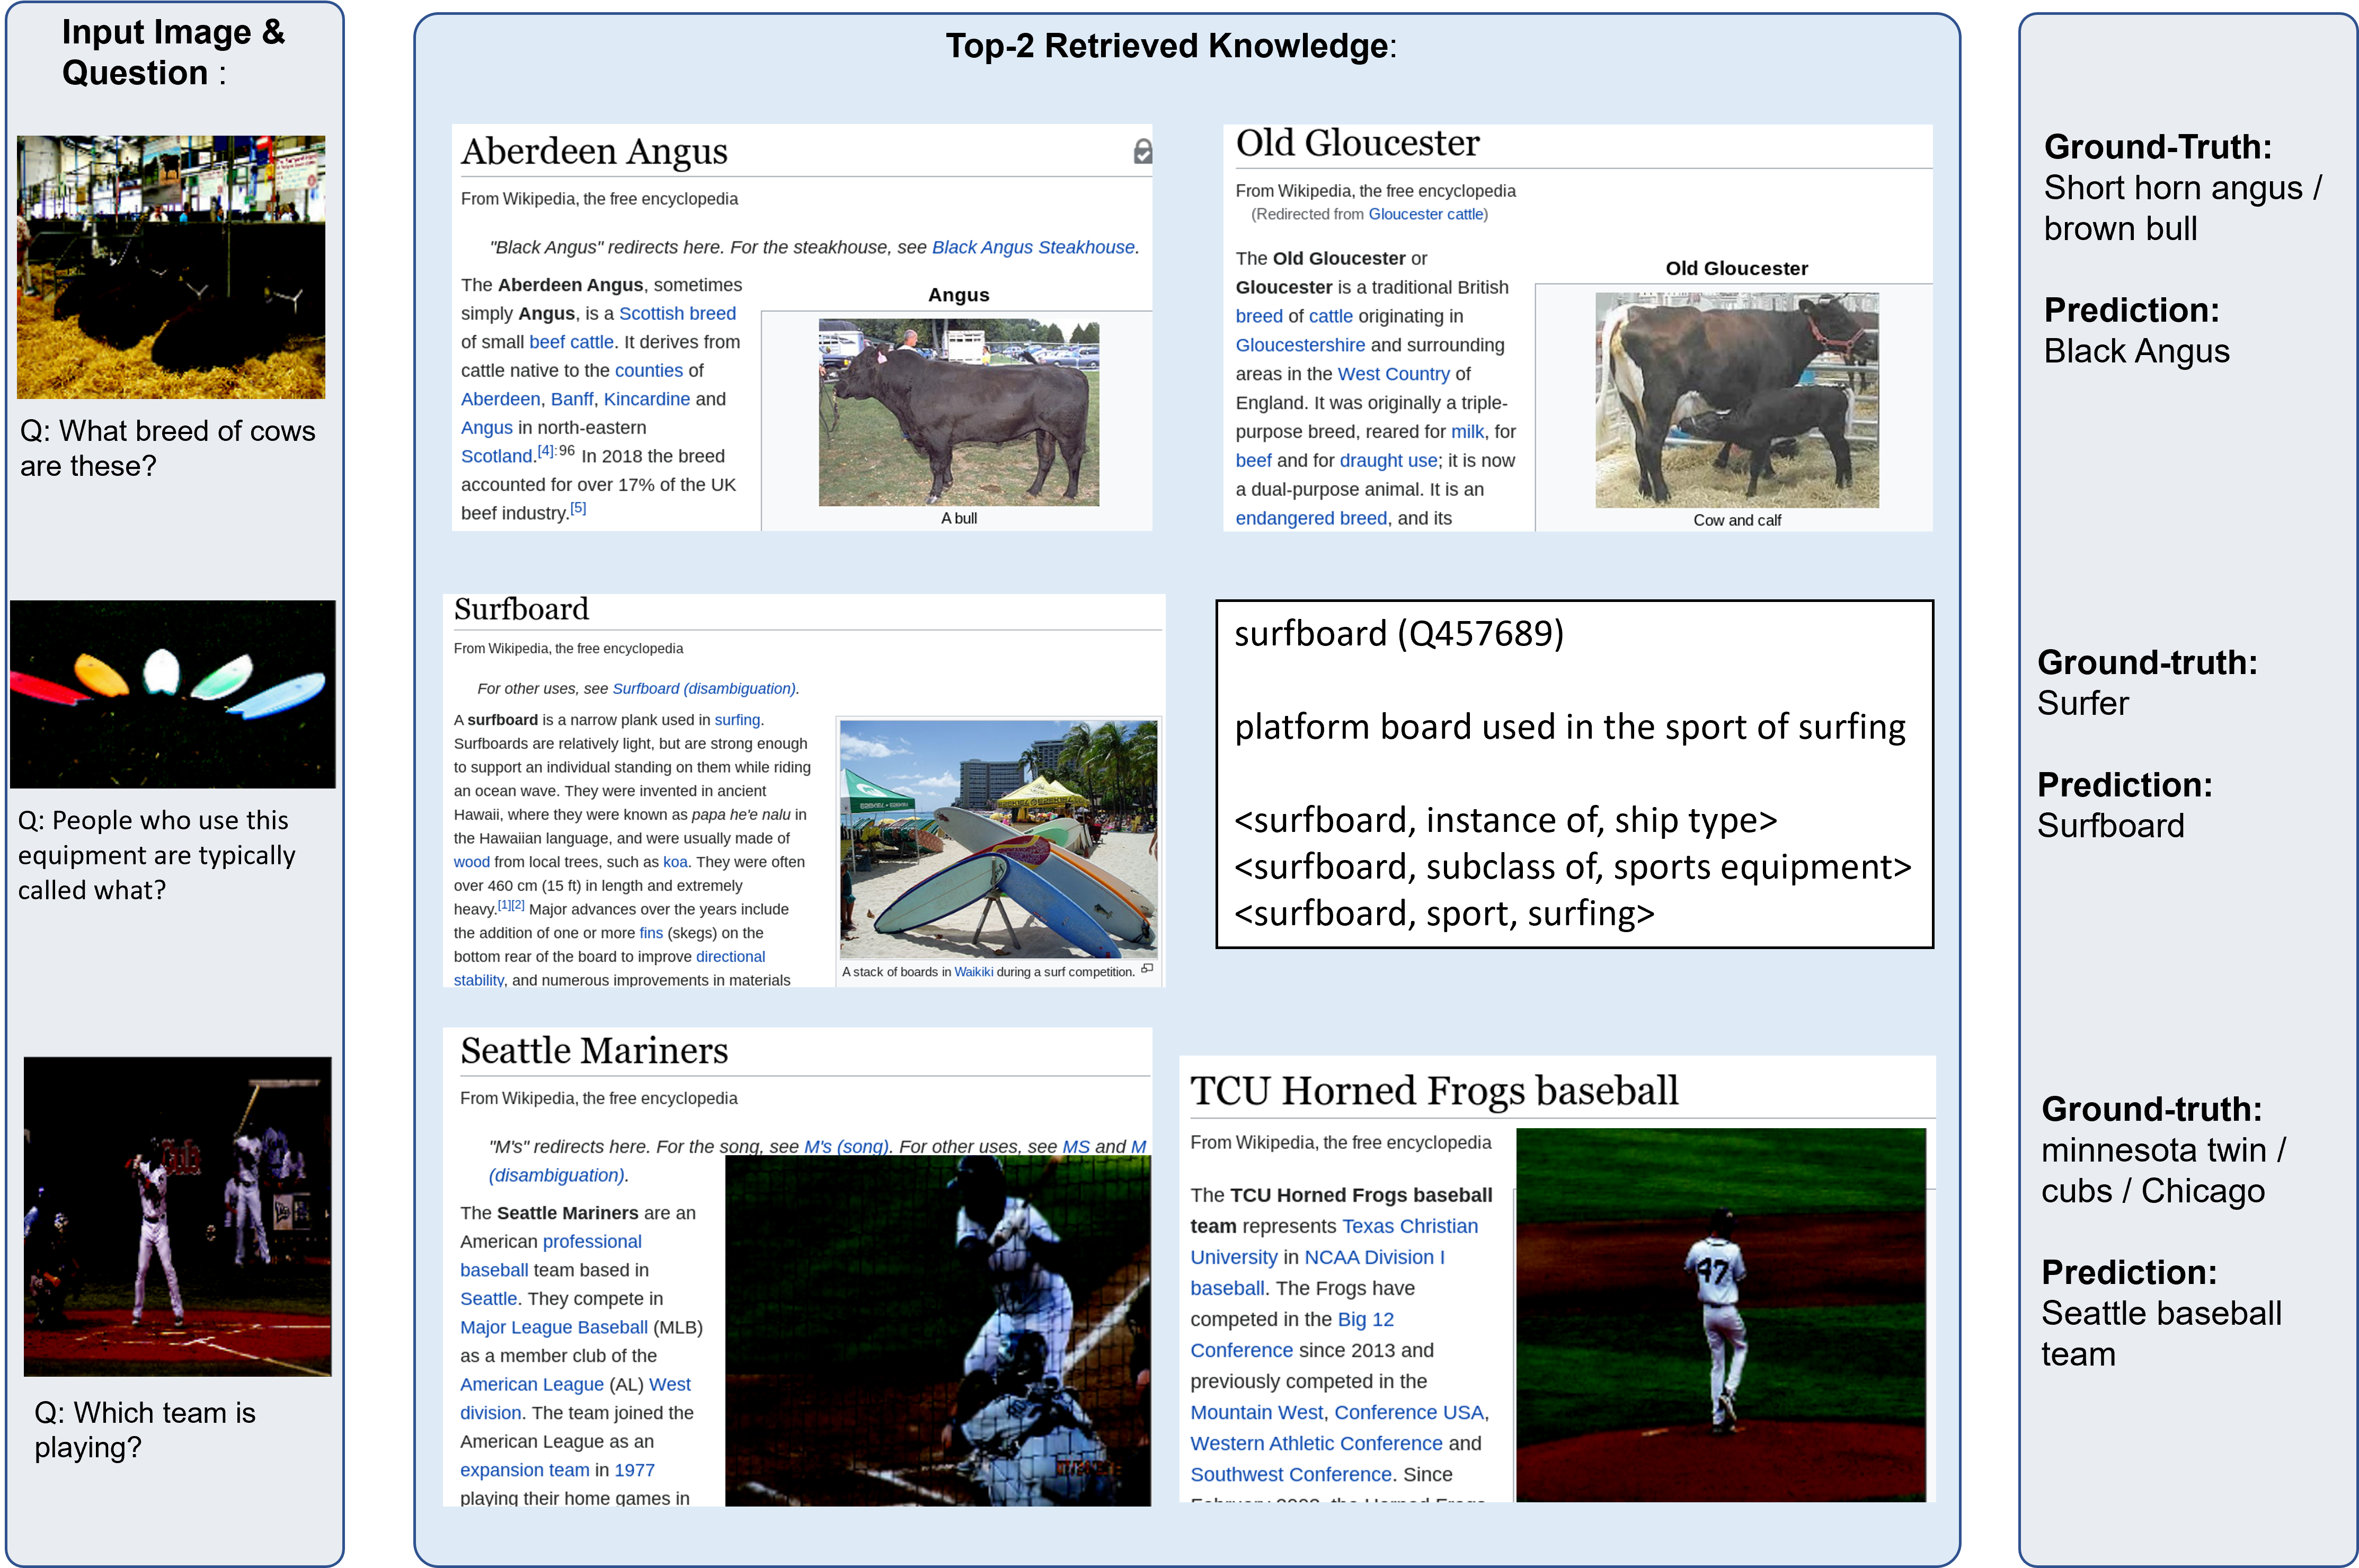}
    \caption{Examples of VQA pairs from OKVQA benchmark that \method make wrong prediction.}
    \label{fig:wrong_vqa}
\end{figure*}

We are also interested to see whether the retrieved knowledge still makes sense for those QA pairs that \method does not make the correct prediction. In Figure~\ref{fig:wrong_vqa} we show such examples. For the first question asking the breed of cows, \method retrieves two species of cow, one from Aberdeen Angus, a formal name for black Angus, and the other is Gloucester. The model's prediction, i.e., ``Black Angus'' is mainly based on the Top-1 retrieved knowledge. Though this prediction is not listed in the ground-truth answers, it is very close to the ground-truth short-horn Angus.
Similarly, in the second question that asks the name of surfing equipment, our model retrieves both the Wikipedia page and Wikidata triplets about surfboard and generates this as the answer. Though it is not exactly the same as a ground-truth answer, i.e., ``surfer'', we think it is another way to say about this equipment. Similar to these two examples, there are many other ones that our model retrieves relevant information but the predicted results are not the same as the ground-truth.
Also there are several examples in which the retrieved knowledge is less useful. For example, in the third question that asks which baseball team is in the image, though our model retrieves several other baseball teams, they are not the same as the ground-truth ones. For these complex questions, it is still space for our model to improve and learn the subtle information from the image to retrieve correct knowledge.

\begin{figure*}
    \centering
    % \vspace{-.2in}
    \includegraphics[width=0.8\columnwidth]{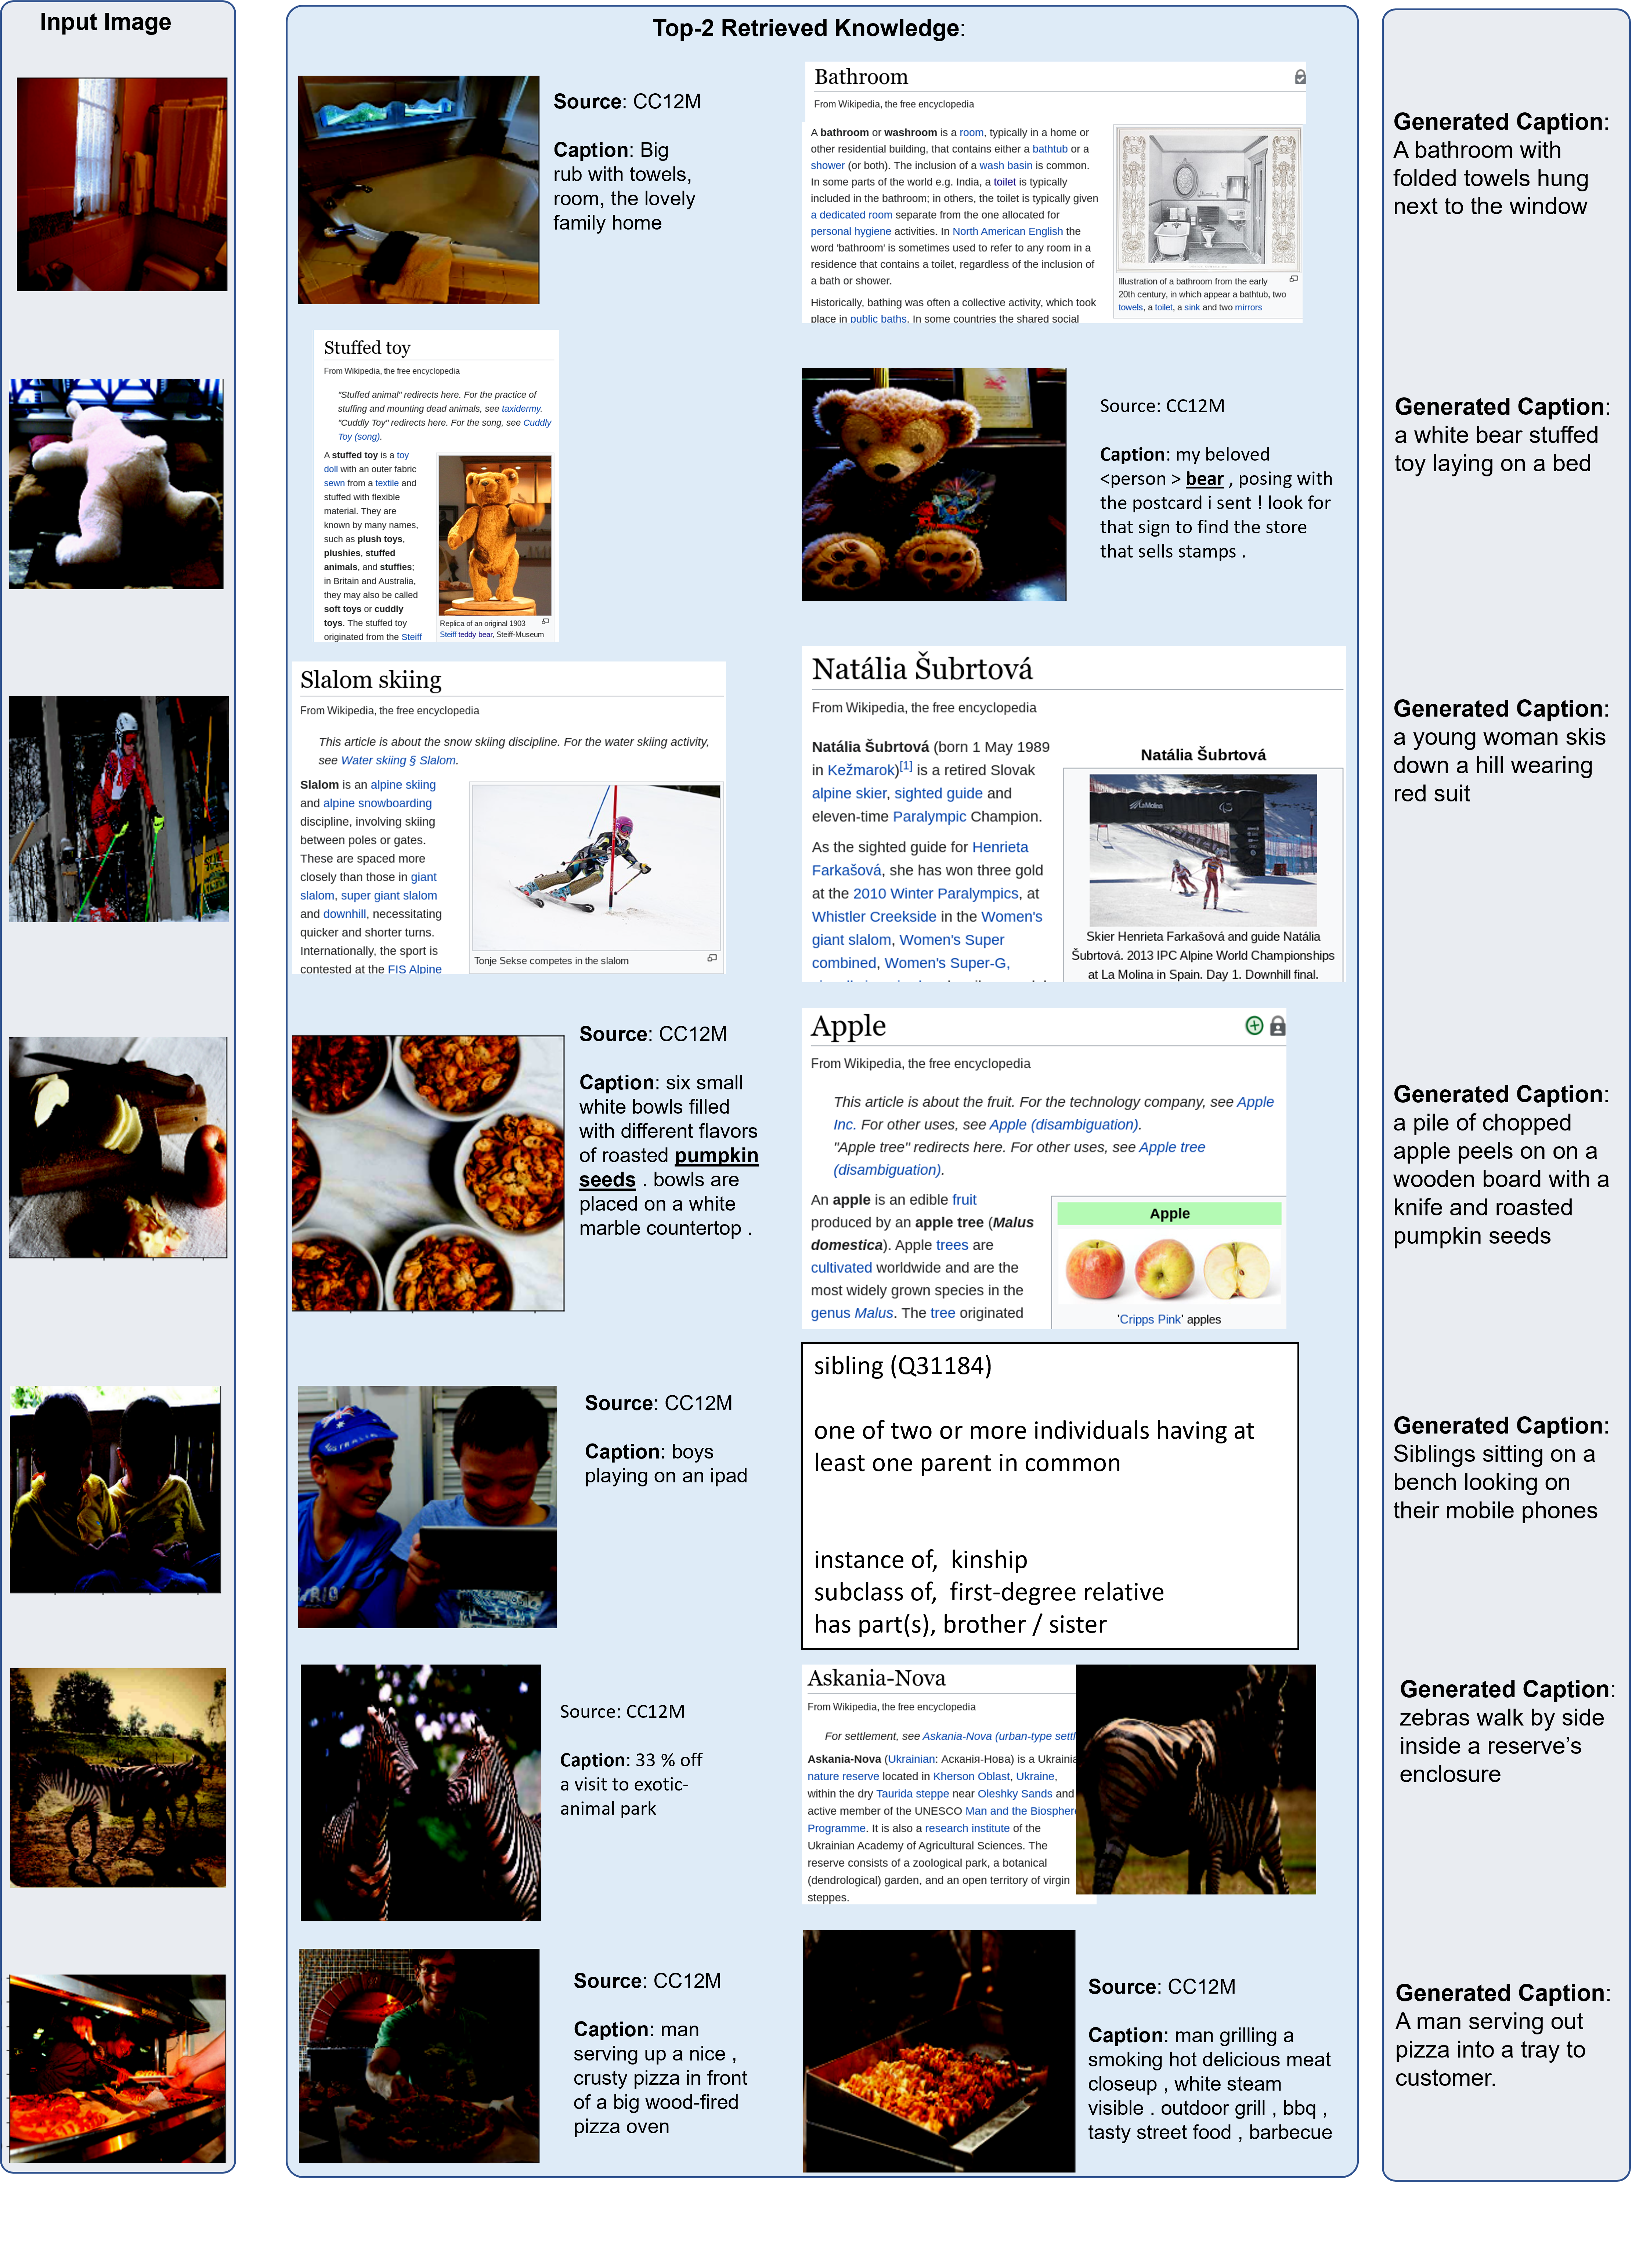}
    \vspace{-.4in}
    \caption{Examples of generated Caption on MSCOCO image captioning dataset.}
    \label{fig:caption}
\end{figure*}

For image captioning, we also show 7 examples in Figure~\ref{fig:caption}. Though image captioning does not rely too much on outside knowledge, our model could still leverage some retrieved knowledge to generate interesting results. In the 5-th example, the model retrieves the definition of sibling, which is a good guess for the relationship between the two kids in the image, and generates sibling in the output caption. In the 6-th example, the model retrieves several knowledge relevant to wildlife reserve, and also generates them. Both the VQA and Image Captioning examples show the effectiveness of the retrieval module for these visual-language tasks.

\section{Hyper-parameter Sensitivity Analysis}
\method consists of two key hyperparameters to achieve good performance: the number of compressed tokens $c$ and the number of retrieved knowledge $K$. We thus conduct sensitivity analysis to investigate how the choice of these two hyperparameters influences final performance.

\begin{table}
\centering
\small
\begin{tabular}{c|cccc} \toprule
\textbf{Setting}  & $K$=10 & $K$=20 & $K$=50 & $K$=100 \\ \midrule
$c=64$ (Pereceiver) &  50.9  & 53.2   & 54.5   & / \\
$c=32$ (Pereceiver)&  51.3  & 53.7   & 54.8   & 55.2 \\
$c=16$ (Pereceiver)&  50.7  & 52.9   & 54.1   & 54.5 \\ \midrule
$c=32$ w/o $\mathcal{L}_{decor}$ &  50.8  & 53.1   & 54.3   & 54.6 \\
$c=32$ w/o $\mathcal{L}_{align}$ &  50.9  & 53.5   & 54.6   & 54.8 \\ \midrule
First $32$ tokens of Encoder & 49.7 & 51.8   & 52.3  & 53.1 \\ \bottomrule
\end{tabular}
\caption{\textbf{Hyperparameter Sensitivity Analysis}: $K$ denotes number of retrieved knowledge entries, and $c$ denotes the number of compressed token for Perceiver model. We also add another naive baseline which simply take the encoder's first $32$ tokens as compression results. Performance is evaluated by fine-tuning a pre-trained \method-Base to OKVQA task.}
\label{tab:hyper}
\end{table}

We take \method-Base architecture, pre-training with different compressed tokens $c \in [16, 32, 64]$ with retrieved knowledge $K=10$. We then fine-tune on downstream OK-VQA datasets with different retrieved knowledge $K \in [10, 20, 50, 100]$. We do not change $K$ during the pre-training stage because of the vast computational cost of pre-training, and we set $K=10$ as a balance between training effectiveness and scalability. While during fine-tuning, it is easy to enumerate different $K$ and study the effects. The results are shown in Table~\ref{tab:hyper}. 

\paragraph{Analyzing number of retrieved knowledge $K$}
From the results, we can first see that increasing number of retrieved knowledge $K$ could consistently improve the performance, and the improvement is not significantly different from 50 and 100. This fits our hypothesis that we require to jointly reason over multiple knowledge to make correct prediction. To strike a balance between performance and efficiency, we choose to use $K=100$ for all fine-tuning tasks.

\paragraph{Analyzing numbers of compressed tokens $c$ }
Regarding value compression, we first compare different numbers of compressed tokens $c$ for the Perceiver model. For each different $c$ we pre-train the \method-Base from scratch and report their fine-tuning results. As is shown in the table, $c=32$ achieves the best performance, even higher than $c=64$. This is probably because $32$ tokens are enough to encode the knowledge information via proper modeling and disentangle regularization. By further increasing the number of tokens, the added capacity will not bring more critical information. Therefore, we choose $c=32$ throughout our study.

\paragraph{Analyzing regularization for Perceiver}
Besides, we also conduct ablation of the two regularization loss we added to guide learning a more informative compression model. we report the result pre-trained without de-correlation loss $\mathcal{L}_{decor}$ and without alignment loss $\mathcal{L}_{align}$. As shown in the second block of the table, each regularization loss plays an important role in the final performance, and incorporating both could lead to optimal performance. 
\paragraph{Another baseline for knowledge compression}
We further add another naive baseline for compression: take the first $32$ tokens from the encoder, i.e., $b(z)[:32]$. As is illustrated, this method performs much worse than Perceiver, probably because the first $32$ tokens in the input sentence are not always the best summarization of the whole knowledge. At the same time, Perceiver could use cross-attention to query the whole sequence properly, and keep the most important information.

\begin{table}
\centering
\small
\begin{tabular}{c|c} \toprule
\textbf{Pre-Training Corpus}  & OKVQA Accuracy \\ \midrule
WIT (5M) &  51.1   \\
\ \ WIT w/o $\mathcal{L}_{contra}$  &  47.6 \\ \midrule
CC12M (12M) &  53.6 \\ 
Web-Image-Text (1.3B) &  55.2 \\ \bottomrule
\end{tabular}
\caption{\textbf{Ablation on Pre-Training Corpus}: We pre-train \method-Base on WIT and CC12M dataset, and report the fine-tuned OKVQA performance.}
\label{tab:corpus}
\end{table}

\begin{table}
\centering
\small
\begin{tabular}{c|cc} \toprule
Setting  & Retrieve from WIT & Retrieve from All \\ \midrule
Frozen ViT &  49.5 & 50.4   \\
Trained ViT &  51.8 & 53.0 \\  \midrule
Ours &  53.1 & 55.2 \\ \bottomrule
\end{tabular}
\caption{\textbf{Compare with Visual-Only Retrieval}: We use ViT-only (frozen or trained) as retriever, retrieve knowledge from WIT or all four corpora.}
\label{tab:vit}
\end{table}

\section{Ablation on Pre-Training Corpus}
Our \method model by default is pre-trained on the 1 billion Web-Image-Text datasets to achieve good performance. Therefore, one natural question is whether the performance improvement relies on the large-scale corpus. We thus also report two results that pre-train our model on WIT and CC12M only. The results are illustrated in Table~\ref{tab:corpus}. As shown, using a much smaller corpus like CC12M for pre-training, the performance is -1.6 lower than the one pre-trained on 1.3B Web-Image-Text dataset. This shows that our retrieval-augmented pre-training framework could still get good results even with a smaller corpus. By scaling up the pre-training corpus, the model could always learn better generation and retrieval results to achieve optimal performance.

We also conduct an ablation study to remove the retrieval warm-start, i.e., $\mathcal{L}_{contra}$ from WIT. This led to a performance drop of -3.5. This matches our intuition that without good initialization for the retrieval module, the retriever would often return irrelevant memory items that would never generate proper training signals, leading to the cold-start problem. Therefore, for all results, we start with a checkpoint pre-trained on WIT with $\mathcal{L}_{contra}$ as a warm-start.

\section{Using Visual-Only Retrieval as Baseline}
in \method we use upper-layer T5 module as both the query Head $\phi_{\texttt{Query}}(\cdot)$ and the key Head $\phi_{\texttt{Key}}(\cdot)$ to compute the query embedding and memory keys. This allow the model using both visual and textual information to conduct retrieval, but requires further training to fuse the two modality. 
In Table 6, we already show that image-to-text matching paradigm (using pre-trained ALIGN) doesn't perform better than our method. 
Another straightforward baseline is to only utilize the visual feature, i.e., only using the ViT embedding output for retrieval. We thus adding two additional baseline, which use the frozen ViT (directly from pre-trained checkpoint without additional training) or trained ViT (using our retrieval-augmented pre-training, but replace the retrieval head with this ViT) for retrieval. As our knowledge corpora also contains some text-only data such as WikiData, for fair comparison, we compare our method with ViT-based retriever by retrieving from WIT or all the four corpora. 
As illustrated in Table~\ref{tab:vit}, using ViT as retriever indeed achieves relatively high performance. When retrieving from WIT and all, the trained ViT only achieve performance -1.3 and -2.2 lower than our image-text model as retriever, and significantly higher than using the ALIGN model for retrieval. This shows that the visual feature plays a very important role for retrieving necessary knowledge. Comparing with the frozen ViT, the trained ViT achieve +2.3 and +2.6 higher performance on the two settings. This shows that our retrieval-augmented training is also useful for getting better retriever, even we directly start from strong ViT checkpoint.

\section{More Implementation Details of Model}
In this section, we provide more details of our model architecture, specifically the Perceiver, Attentive fusion module and online distributed MIPS retrieval.

\subsection{Perceiver as Value Compression Head}
As we described in the method section of the submission, we propose to compress the full token embedding sequence into a shorter sequence by using the Perceiver model~\cite{DBLP:conf/icml/JaegleGBVZC21}.

Perceiver is a standard Transformer Decoder model that uses a learnable latent embedding $\texttt{Emb}_{\texttt{Latent}}$ as input query, and the full embedding sequence to be compressed $b(z)$ as key and value. For each layer, the perceiver first uses a cross-attention module to compress a $l$-length full embedding sequence $b(z) \in \mathbb{R}^{I \times d}$ into the $c$-length queries by $\texttt{Emb}_{\texttt{Latent}} \in \mathbb{R}^{c \times d}$, followed by self-attention in the latent space. We write the full compression operation as below:
\begin{algorithm}[th]
  \caption{Perceiver Operation ($\psi(\cdot)$)}
  \label{alg:main}
\begin{algorithmic}
  \STATE {\bfseries Input:} $Z^0 = \texttt{Emb}_{\texttt{Latent}} \in \mathbb{R}^{c \times d}$,
  \STATE $B = \text{LayerNorm}(b(z))  \in \mathbb{R}^{I \times d}$
  \FOR{layer $l$ for each Perceiver layers}
    \STATE $\hat{Z}^{l} = \text{LayerNorm}(Z^{l-1})$
    \STATE $\hat{Z}^{l} = \text{Cross-Attn}\big(\text{Query=}\hat{Z}^{l}, \text{Key\&Value=}B\big) + Z^{l-1}$
    \STATE $\hat{Z}^{l} = \text{Self-Attention}\big(\text{LayerNorm}(\hat{Z}^{l})\big)+\hat{Z}^{l}$
    \STATE $Z^{l} = \text{MLP}\big(\text{LayerNorm}(\hat{Z}^{l})\big)+\hat{Z}^{l}$
  \ENDFOR
  \STATE {\bfseries Return:}  $\psi(b(z)) = Z^{L} \in \mathbb{R}^{c \times d}$ 
\end{algorithmic}
\end{algorithm}

We denote $Z^{l}$ as $l$-th layer's output, and $\hat{Z}^{l}$ as intermediate representation. 
After stacking $L$ Perceiver layers, we could learn a meaningful short $c$-length compressed embedding sequence $Z^{L}$ to represent the original full sequence. To implement Perceiver that is consistent with the remaining model architecture, we use the standard T5 Decoder with randomly initialized latent embedding $\texttt{Emb}_{\texttt{Latent}}$. 

\section{Attentive Fusion}
In this section, we provide more details about the Attentive fusion module in our model. The attentive fusion module aims to allow end-to-end training of the retriever and generator weights. Without this fusion module, the retriever is not involved in the final answer generation procedure and will not receive gradients. Some of the previous work~\cite{DBLP:journals/corr/abs-2002-08909,DBLP:conf/nips/LewisPPPKGKLYR020,DBLP:conf/nips/SachanRHDY21F} utilize alternative training signals for updating retriever. They conduct generation using one knowledge entry at a time instead of using all Top-K and use the corresponding generation accuracy as the training signal. This approach is not guaranteed to be optimal for multi-knowledge retrieval. It is also very inefficient if we want to retrieve up-to-hundred knowledge items.

Our solution is to inject the retrieval score as a soft attention mask into the fusion and decoding process, as is illustrated in Figure~\ref{fig:fusion}. At each Transformer Layer before attention calculation, we multiply the retrieval probability $p(z_i|x)$ to each token embedding belonging to knowledge $z_i$. 
We denote the concatenated query embedding and memory values as $X = [b(x), \psi(b(z_1)), \dots, \psi(b(z_K))] \in \mathbb{R}^{(I + c \cdot K) \times d}$, where $I$ is the number of tokens of the input query $x$ and $c$ is the number of compressed tokens.
Based on the top-$K$ retrieved knowledge $Z = [z_1, \cdots, z_K]$ with key and value embeddings, we could calculate the probability over these top-$K$ knowledge similar to eq.(3):
\begin{align}
    p(z_i \mid x) =  &  \frac{\exp  \big( Gate_{\mathcal{MI}(z_i)}(x) \cdot Rel(x, z_i) / \tau \big) }{\sum_{j=1}^K \exp\big( Gate_{\mathcal{MI}(z_j)}(x) \cdot Rel(x, z_j) / \tau \big)}, \nonumber \\
\end{align}
\begin{align}
    \text{where}\ \ Rel(x,z_i) & = \texttt{Emb}_{\texttt{Query}}(x)^T \cdot \texttt{Emb}_{\texttt{Key}}(z_i) \\
    & = \phi_{\texttt{Query}}(b(x))^T \cdot \phi_{\texttt{Key}}(b(z_i))
\end{align}
Here we denote $\mathcal{MI}(z_i)$ as the indicator function returning corpus ID of retrieved knowledge $z_i$, such that $\mathcal{M}^j = \mathcal{MI}(z_i^j)$. Note that the difference of this probablity within Top-K results differ with eq.(\ref{eq:prob}) in that we only summing over the $K$ subset results, and also we merge the gating score into the softmax to make the output a probability that summing to one.
We then construct a latent soft attention mask over $X$ as:
\begin{align}
\texttt{Mask}_{\texttt{att}} = \Big[ &  \big[ \underbrace{ 1,\cdots, 1 }_{\text{repeat} \times l}\big], \ \big[\underbrace{ p(z_1 \mid x),\cdots, p(z_1 \mid x) }_{\text{repeat} \times c}\big], \ \dots, \nonumber \\
\dots,\ & \big[\underbrace{ p(z_K \mid x), \cdots, p(z_K \mid x) }_{\text{repeat} \times c}\big] \Big]. \label{eq:mask}
\end{align}
Then, within the attentive fusion module, we multiply this attention mask $\texttt{Mask}_{\texttt{att}}$ to the whole embedding sequence. We write the full attentive fusion operation as below:
\begin{algorithm}[th]
  \caption{Attentive Fusion Operation ($F(\cdot)$}
  \label{alg:main}
\begin{algorithmic}
  \STATE {\bfseries Input:} $X^{0} = [b(x), \psi(b(z_1)), \dots, \psi(b(z_K))]$,
  \STATE \textbf{Calculate} $\texttt{Mask}_{\texttt{att}} \in \mathbb{R}^{(I + c \cdot K) \times 1}$ following Eq.(\ref{eq:mask}),
  \FOR{layer $l$ for each Fusion layers}
    \STATE $\hat{X}^{l} = \texttt{Mask}_{\texttt{att}} \cdot \text{LayerNorm}(X^{l-1}) \label{eq:fusion}$
    \STATE $\hat{X}^{l} = \text{Self-Attention}(\hat{X}^{l}) + X^{l-1}$
    \STATE $X^{l} = \text{MLP}\big(\text{LayerNorm}(\hat{X}^{l})\big) + \hat{X}^{l} $
  \ENDFOR
  \STATE {\bfseries Return:}  $F(X) = X^{L} \in \mathbb{R}^{(I + c \cdot K) \times d}$ 
\end{algorithmic}
\end{algorithm}

We denote $X^{l}$ as $l-$th layer's output, and $\hat{X}^{l}$ as intermediate representation. 
The critical difference is shown in eq.(\ref{eq:fusion}), in which we multiply $\texttt{Mask}_{\texttt{att}}$ to the pre-normalized representation (T5 utilizes pre-norm which satisfies our purpose). In this way, when we calculate the attention within the self-attention operation, the attention scores each knowledge sends to other position $a_{:,i}$ is proportional to $p(z_i|x)$. This reflects the importance of this knowledge $z_i$ to make the final prediction. By multiplying the retrieval score as prior and through end-to-end training, the retriever could be learned to identify those samples that are more important to final output generation. This is similar to adopting a posterior estimation $p(z|x,y)$, which takes output answer $y$ as condition, to optimize the retriever model better.

This modified retrieval injected fusion layer is also similar to the Mixture-of-Expert (MOE) model, in which the retrieval is like a gating layer to select knowledge, and the knowledge representation serves as the expert. In this way, we turn the discrete knowledge retrieval/selection learning into a continuous learning problem, and the whole model could be learned end-to-end.

\subsection{Online Distributed MIPS Retrieval}
To strike a balance between training efficiency and scalability, we store the key embedding memory on TPU, and store the value sequence embeddings (each sequence contains $c=32$ token embeddings) and raw dataset in the local host's CPU memory. Then, when doing retrieval, each device first conduct MIPS operation over on-device memory to find local Top-K entry ID, then syncs the results across TPU devices to get global Top-K, and then returns the corresponding results. The detailed procedure is as follows:

\begin{algorithm}[th]
 \caption{Online Distributed MIPS Retrieval}
  \label{alg:main}
\begin{algorithmic}
  \STATE {\bfseries Input:} Batch query $\texttt{Emb}_{\texttt{Query}} \in \mathbb{R}^{\text{bsz} \times d}$, Local On-TPU key embeddings $\texttt{Key}(\mathcal{M}) \in \mathbb{R}^{|\mathcal{M}| \times d}$, Local On-CPU values $\texttt{DB}(\mathcal{M})$.
  \STATE \textbf{For each TPU device:}
  \STATE $\hat{\texttt{Emb}}_{\texttt{Query}}=\text{Gather}(\texttt{Emb}_{\texttt{Query}})$
  \STATE $local\_scores =\hat{\texttt{Emb}}_{\texttt{Query}}^T\cdot \texttt{Emb}_{\texttt{Key}}(\mathcal{M})$ 
  \STATE $local\_ids = \text{Approx\_Top\_K}(local\_scores)$
  \STATE $local\_vals = \texttt{DB}(\mathcal{M}).\text{Lookup}(local\_ids)$
  \STATE $global\_scores = \text{Gather}(local\_scores)$
  \STATE $global\_ids = \text{Top\_K}(global\_scores)$
  \STATE {\bfseries Return:}  $\text{Gather}(local\_scores).\text{Batch\_Select}(global\_ids)$ 
\end{algorithmic}
\end{algorithm}

This distributed retrieval could be done in a hierarchical manner if we group multiple TPUs into the same host, so we could first find Top-K by syncing within each host, and then syncing across host to find global Top-K, which further reduce the communication redundancy.
